# Supplementary material for: Action tube generation by person query matching for spatio-temporal action detection
Source: arXiv:2503.12969 source file (2025-03-17)
Supplement: Supplementary file 1 [file appendix.tex]

\setcounter{figure}{0}
\setcounter{table}{0}

\section{なにかの追加の説明}

＊＊＊＊＊＊＊＊＊＊＊＊＊＊＊＊
＊＊＊＊＊＊＊＊＊＊＊＊＊＊＊＊
＊＊＊＊＊＊＊＊＊＊＊＊＊＊＊＊
＊＊＊＊＊＊＊＊＊＊＊＊＊＊＊＊
＊＊＊＊＊＊＊＊＊＊＊＊＊＊＊＊
